# Supplementary material for: Outdoor Scene Extrapolation with Hierarchical Generative Cellular Automata
Source: arXiv:2406.08292 source file (2024-06-12)
Supplement: Supplementary file 1 [file main_appendix.tex]

% CVPR 2024 Paper Template; see https://github.com/cvpr-org/author-kit

\documentclass[10pt,twocolumn,letterpaper]{article}

%%%%%%%%% PAPER TYPE  - PLEASE UPDATE FOR FINAL VERSION
\usepackage{cvpr}              % To produce the CAMERA-READY version
% \usepackage[review]{cvpr}      % To produce the REVIEW version
% \usepackage[pagenumbers]{cvpr} % To force page numbers, e.g. for an arXiv version

% Import additional packages in the preamble file, before hyperref
\input{preamble}

% It is strongly recommended to use hyperref, especially for the review version.
% hyperref with option pagebackref eases the reviewers' job.
% Please disable hyperref *only* if you encounter grave issues, 
% e.g. with the file validation for the camera-ready version.
%
% If you comment hyperref and then uncomment it, you should delete *.aux before re-running LaTeX.
% (Or just hit 'q' on the first LaTeX run, let it finish, and you should be clear).
\definecolor{cvprblue}{rgb}{0.21,0.49,0.74}
\usepackage[pagebackref,breaklinks,colorlinks,citecolor=cvprblue]{hyperref}
\usepackage{url}

\usepackage[utf8]{inputenc} % allow utf-8 input
\usepackage[T1]{fontenc}    % use 8-bit T1 fonts
\usepackage{booktabs}       % professional-quality tables
\usepackage{amsfonts}       % blackboard math symbols
\usepackage{nicefrac}       % compact symbols for 1/2, etc.
\usepackage{microtype}      % microtypography
\usepackage{xcolor}         % colors
\usepackage{amsthm}
\usepackage{amsmath}
\usepackage{amssymb}
\usepackage{dsfont}
\usepackage{amsthm}
\usepackage{thm-restate}
\usepackage{graphicx}
\usepackage{blindtext}
\usepackage{multirow}
\usepackage{gensymb}
\usepackage{float}
\usepackage{caption}
\usepackage{amssymb}% http://ctan.org/pkg/amssymb
\usepackage{pifont}% http://ctan.org/pkg/pifont
\usepackage{hyperref}
\usepackage{textcomp}

%
%

%%%%%%%%% PAPER ID  - PLEASE UPDATE
 % *** Enter the Paper ID here

%%%%%%%%% TITLE - PLEASE UPDATE
\title{
Supplementary Material for \\
Outdoor Scene Extrapolation with \\
Hierarchical Generative Cellular Automata
}

%%%%%%%%% AUTHORS - PLEASE UPDATE
% \author{First Author\\
% Institution1\\
% Institution1 address\\
% {\tt\small firstauthor@i1.org}
% % For a paper whose authors are all at the same institution,
% % omit the following lines up until the closing ``}''.
% % Additional authors and addresses can be added with ``\and'',
% % just like the second author.
% % To save space, use either the email address or home page, not both
% \and
% Second Author\\
% Institution2\\
% First line of institution2 address\\
% {\tt\small secondauthor@i2.org}
% }

\begin{document}

\twocolumn[{
\renewcommand\twocolumn[1][]{#1}

\maketitle

}]

% reduces space around equations
\setlength{\abovedisplayskip}{2pt}
\setlength{\belowdisplayskip}{3pt}

% \begin{abstract}
% \vspace{-3.5mm}
% \input{00_abstract}
% \end{abstract}
% 
% \input{01_intro}
% \input{02_related_works}
% \input{04_hgca}
% \input{05_experiments}
% \input{06_conclusion}
% We additionally include generation process video on synthetic scene (\texttt{karton.mp4}) and real-world scene (\texttt{waymo.mp4}) of hGCA in the supplementary material for further visualization.

\appendix
\input{08_appendix}
{
    \small
    \bibliographystyle{ieeenat_fullname}
    \bibliography{main}
}

% WARNING: do not forget to delete the supplementary pages from your submission 
% \input{sec/X_suppl}

\end{document}
